# Supplementary material for: Manifestation of dipole-induced disorder in self-assembly of ferroelectric and ferromagnetic nanocubes
Source: arXiv:1903.08411 source file (2019-03-20)
Supplement: Supplementary file 1 [file supplemental.pdf]

SUPPLEMENTAL INFORMATION

# Manifestation of dipole-induced disorder in self-assembly of ferroelectric and ferromagnetic nanocubes

Dmitry Zablotsky,[a,b] Leonid L. Rusevich,[a] Guntars Zvejnieks,[a] Vladimir Kuzovkov,[a] and Eugene Kotomin[a,c]

[a] Institute of Solid State Physics, Kengaraga str. 8, LV-1063 Riga, Latvia.
[b] University of Latvia, Raina bulv. 19, LV-1586 Riga, Latvia. E-mail: dmitrijs.zablockis@lu.lv
[c] Max Planck Institute for Solid State Research, Heisenbergstr. 1, 70569 Stuttgart, Germany. E-mail: kotomin@fkf.mpg.de

## Quantum-chemical computations

First-principles (*ab initio*) quantum-chemical simulations are performed within the linear combination of atomic orbitals (LCAO) approximation and partially periodic boundary conditions, using advanced hybrid functionals of the density-functional-theory (DFT). The CRYSTAL code (v.14) [1] was used to calculate dipole moments for stoichiometric isolated slabs of $BaTiO_3$ and $SrTiO_3$. Calculations have been performed with PBE0 hybrid DFT-HF exchange-correlation functional [2] combining the Perdew–Burke-Ernzerhof (PBE) exchange functional with 25% of the Hartree-Fock (HF) exchange and the PBE correlation functional, which already proved reliable for piezoelectric properties. [3][4][5].

The inner core orbitals of Ba, Sr and Ti atoms were described using Hay and Wadt effective small-core pseudopotentials (ECP) [6][7][8], the outer core $5s^2 5p^6 6s^2$ sub-valence and valence electrons for Ba, $4s^2 4p^6 5s^2$ electrons for Sr and $3s^2 3p^6 3d^2 4s^2$ for Ti are calculated self-consistently. The oxygen atoms were described by an all-electron basis set. The basis sets for Ba, Sr and Ti were reused from Ref. [9], where they were previously optimized for $BaTiO_3$ and $SrTiO_3$ crystals, whereas the basis set for oxygen was adopted from Ref. [10].

Our computational set up has been calibrated in terms of accuracy and computational time. The cut-off thresholds governing the truncation of infinite coulomb and exchange lattice sums in the two-electron integral evaluation have been set to 8, 8, 8, 8, 16, and a regular Monkorst-Pack mesh of points in reciprocal space has been used, whose shrinking factor has been set to 12, while the convergence threshold on total energy was set to $10^{-10}$ Ha (Hartree) for self-consistent field (SCF) calculations and geometry optimization. These parameters ensure converged results.

A partially periodic isolated slab structure was cut from the prototype 3D $BaTiO_3$/$SrTiO_3$ cubic crystal (SG 221, $BaTiO_3$: a=3.993 Å, $SrTiO_3$: a=3.901 Å) along <100> crystallographic planes, with AO (where A = Ba or Sr) and $TiO_2$ terminations [11]. We have calculated the dipole moments for $BaTiO_3$ and $SrTiO_3$ stoichiometric slabs of different thicknesses specified in Table 2.

**Table 2.** The values of the dipole moment perpendicular to the slab (along *z*-axis) depending on number of unit cells along *z*-axis in the initial structure (thickness of slab), *n* — number of unit cells along z-axis; *a*=*b* — calculated in-plane lattice constants (perpendicular to *z*-axis)

| | $BaTiO_3$ | | $SrTiO_3$ | |
|---|---|---|---|---|
| *n* | *a*=*b*, Å | Dip. moment, D | *a*=*b*, Å | Dip. moment, D |
| 3 | 3.947 | 2.0338 | 3.866 | 1.3177 |
| 4 | 3.958 | 2.0553 | 3.874 | 1.3285 |

| | | | | |
|---|---|---|---|---|
| 5 | 3.965 | 2.0620 | 3.879 | 1.3306 |
| 6 | 3.970 | 2.0649 | 3.883 | 1.3291 |

**P$^3$M implementation**

Here a brief summary of the treatment of long-ranged dipolar interaction in the NPT self-assembly simulations is presented for reference. The dipole-dipole interaction [12] between two point dipoles $\boldsymbol{\mu}_i$ and $\boldsymbol{\mu}_j$ placed at $\boldsymbol{r_i}$ and $\boldsymbol{r_j}$ and separated by a distance $r_{ij} = |\mathbf{r}_i - \mathbf{r}_j|$

$$\beta U_{dd}(\boldsymbol{\mu_i}, \boldsymbol{\mu_j}, \boldsymbol{r_{ij}}) = \lambda(\hat{\boldsymbol{\mu}}_i \cdot \nabla_{r_i})(\hat{\boldsymbol{\mu}}_j \cdot \nabla_{r_j})\frac{1}{|\boldsymbol{r}_{ij}|} = -\frac{\lambda}{r_{ij}^3}[3(\hat{\boldsymbol{\mu}}_i \cdot \hat{\boldsymbol{r}}_{ij})(\hat{\boldsymbol{\mu}}_j \cdot \hat{\boldsymbol{r}}_{ij}) - \hat{\boldsymbol{\mu}}_i \cdot \hat{\boldsymbol{\mu}}_j]$$

The total energy of a system of N point dipoles $\{\boldsymbol{\mu}_i\}_{i=1}^N$ with positions $\{\mathbf{r}_i\}_{i=1}^N$ in a periodic simulation box defined by edge vectors $\mathbf{a} = \{\mathbf{a_1} \quad \mathbf{a_2} \quad \mathbf{a_3}\}$ (as columns)

$$\beta U = \frac{1}{2}\sum_{\mathbf{n}}{}' \sum_{i=1}^{N}\sum_{j=1}^{N} \beta U_{dd}(\hat{\boldsymbol{\mu}}_i, \hat{\boldsymbol{\mu}}_j, \mathbf{r}_{ij} + \mathbf{Ln})$$

where $\mathbf{L} \equiv \mathrm{diag}(|\mathbf{a_1}|, |\mathbf{a_2}|, |\mathbf{a_3}|)$ and the sum runs over the periodic images of the system indexed by $\mathbf{n} = (n_1, n_2, n_3)$ with $n_\beta \in \mathbb{Z}$ and the prime indicates that the term with $i = j$ is omitted for $\mathbf{n} = 0$. The dipolar sum is conditionally convergent [13], using Ewald decomposition the long-ranged dipolar interaction is split into a short-range component $U^{(r)}$, which is evaluated in real space, and a long-range part $U^{(k)}$, which is calculated in Fourier space. Due to its fast decay the former can be treated efficiently within a conventional MD framework. The real-space part of the energy, force and torque on a dipole $i$ are accordingly [14][15][16]

$$U^{(r)} = \frac{1}{2}\sum_{\mathbf{n}}{}' \sum_{i=1}^{N}\sum_{j=1}^{N}\{(\boldsymbol{\mu}_i \cdot \boldsymbol{\mu}_j)B(|\boldsymbol{r}_{ij} + \mathbf{n}|) - [\boldsymbol{\mu}_i \cdot (\mathbf{r}_{ij} + \mathbf{n})][\boldsymbol{\mu}_j \cdot (\mathbf{r}_{ij} + \mathbf{n})]C(|\mathbf{r}_{ij} + \mathbf{n}|)\}$$

$$\mathbf{F}_{ij}^{(r)}(\boldsymbol{r_{ij}}) = \{[(\boldsymbol{\mu}_\mathrm{i} \cdot \boldsymbol{\mu}_\mathrm{j})\mathbf{r}_\mathrm{ij} + \boldsymbol{\mu}_\mathrm{i}(\boldsymbol{\mu}_\mathrm{j} \cdot \mathbf{r}_\mathrm{ij}) + (\boldsymbol{\mu}_\mathrm{i} \cdot \mathbf{r}_\mathrm{ij})\boldsymbol{\mu}_\mathrm{j}]C(r_{ij}) - (\boldsymbol{\mu}_\mathrm{i} \cdot \mathbf{r}_\mathrm{ij})(\boldsymbol{\mu}_\mathrm{j} \cdot \mathbf{r}_\mathrm{ij})D(r_{ij})\mathbf{r_{ij}}\}$$

$$\boldsymbol{\tau}_{ij}^{(r)}(\boldsymbol{r_{ij}}) = -\sum_{\mathbf{n}}{}' \sum_{j=1}^{N}(\boldsymbol{\mu}_\mathrm{i} \times \boldsymbol{\mu}_\mathrm{j})B(r_{ij}) - (\boldsymbol{\mu}_\mathrm{i} \times \mathbf{r}_\mathrm{ij})(\boldsymbol{\mu}_\mathrm{j} \cdot \mathbf{r}_\mathrm{ij})C(r_{ij})$$

where the real-space coefficients

$$B(r) = \frac{1}{r^3}\left[\mathrm{erfc}(\alpha r) + \frac{2\alpha r}{\sqrt{\pi}}e^{-\alpha^2 r^2}\right]$$

$$C(r) = \frac{1}{r^5}\left[3\,\mathrm{erfc}(\alpha r) + \frac{2\alpha r}{\sqrt{\pi}}(3 + 2\alpha^2 r^2)e^{-\alpha^2 r^2}\right] = \frac{1}{r^2}\left[3B(r) + \frac{4\alpha^3}{\sqrt{\pi}}e^{-\alpha^2 r^2}\right]$$

$$D(r) = \frac{1}{r^7}\left[15\,\mathrm{erfc}(\alpha r) + \frac{2\alpha r}{\sqrt{\pi}}(15 + 10\alpha^2 r^2 + 4\alpha^4 r^4)e^{-\alpha^2 r^2}\right] = \frac{1}{r^2}\left[5C(r) + \frac{8\alpha^5}{\sqrt{\pi}}e^{-\alpha^2 r^2}\right]$$

and the Ewald splitting parameter $\alpha$ determines their effective range.

In turn, the long-range contribution is short-ranged in Fourier space and is summed there with metallic boundary conditions [15][17]

$$U^{(k)} = \frac{1}{2V}\sum_{\mathbf{k}\neq 0}|\hat{\boldsymbol{\rho}}(\boldsymbol{k})\cdot i\mathbf{k}|^2\,\hat{G}_{\mathbf{k}} - \frac{2\alpha^3}{3\sqrt{\pi}}\sum_{i=1}^{N}\boldsymbol{\mu}_i^2 \qquad \text{(S1)}$$

where $V = \det \boldsymbol{a}$ is the volume of the simulation box, the wave vector $\mathbf{k} \equiv \{2\pi\mathbf{m}^T\mathbf{a}^{-1}\colon \mathbf{m} \in \mathbb{Z}^{\mathbf{3}}\}$ and $\mathbf{a}^{-1} = \{\boldsymbol{a}_1^* \quad \boldsymbol{a}_2^* \quad \boldsymbol{a}_3^*\}^{\mathrm{T}}$ having reciprocal vectors as rows; $\hat{\boldsymbol{\rho}}(\mathbf{k})$ is the Fourier transform of the periodic dipole density distribution $\boldsymbol{\rho}(\mathbf{r}) = \sum_{i=1}^{N}\boldsymbol{\mu}_i\,\delta(\mathbf{r}-\mathbf{r}_i)$

$$\hat{\boldsymbol{\rho}}(\mathbf{k}) = \mathrm{FT}[\boldsymbol{\rho}](\mathbf{k}) = \sum_{i=1}^{N}\boldsymbol{\mu}_i\,e^{-i\mathbf{k}\cdot\mathbf{r}_i}$$

and the Green (influence) function

$$\hat{G}(\mathbf{k}) = \mathrm{FT}[\mathrm{erf}(\alpha r)\,r^{-1}](\mathbf{k}) = \frac{4\pi}{|\mathbf{k}|^2}e^{-|\mathbf{k}|^2/4\alpha^2}$$

In the particle-particle-particle-mesh ($P^3M$) Ewald method [18] the fast Fourier transform (FFT) is used to accelerate the calculation of the **k**-space component, which is the optimal approach for systems of moderate size ($300<N<10^5$ particles) [17][19].

Hence, the simulation domain is discretized by a $\mathbf{N} \equiv \mathrm{diag}(N_1, N_2, N_3)$ mesh with spacing $\mathbf{H} \equiv \mathrm{diag}(h_1, h_2, h_3) = \mathbf{N}^{-1}\mathbf{L}$, where the mesh points are identified by lattice vectors $\mathbf{r}_{\boldsymbol{m}} \equiv \{(\mathbf{aN}^{-1})\mathbf{n}\colon \mathbf{n} \in \mathbb{Z}^3, 0 \le n_\beta < N_\beta\}$.

The point dipoles are mapped onto a mesh-based dipole density distribution by *p*-order assignment functions $W^{(p)}$, which distribute the dipole onto the nearest mesh points

$$\boldsymbol{\rho}_{\mathbf{r}_m} = \frac{1}{|\mathbf{H}|}\sum_{i=1}^{N}\boldsymbol{\mu}_i W^{(p)}(\mathbf{r}_{\boldsymbol{m}} - \mathbf{r}_{\boldsymbol{i}})$$

where $\mathbf{r}_{\boldsymbol{i}}$ is the coordinate of particle $i$; $W^{(p)}(\mathbf{r}) = w^{(p)}(s_1)w^{(p)}(s_2)w^{(p)}(s_3)$ and $w^{(p)}$ are shifted B-splines over the nearest p mesh points (per coordinate direction) over the interval $[-0.5p,\ 0.5p]$, $\mathbf{s} = \mathbf{Na}^{-1}\mathbf{r}$ are scaled coordinates $s_\beta \in [0, N_\beta]$ along directions $\mathbf{a}_\beta$ [18][20][17][19]. The Fourier coefficients of the mesh-based dipole density are calculated using the FFT

$$\hat{\boldsymbol{\rho}}_{\mathbf{k}_\mathrm{n}} = \mathrm{FFT}\{\boldsymbol{\rho}_{\mathbf{r}_m}\}(\mathbf{k}_\mathrm{n}) = \frac{1}{V}\sum_{\mathbf{r}_m} e^{i\mathbf{k}_\mathbf{n}\cdot\mathbf{r}_m}\boldsymbol{\rho}_{\mathbf{r}_\mathbf{m}}$$

over the set of wave vectors in one Brillouin zone $\mathbf{k}_\mathrm{n} \equiv \{2\pi\mathbf{n}^\mathrm{T}\mathbf{a}^{-1}\colon \mathbf{n} \in \mathbb{Z}^{\mathbf{3}}, |n_\beta| < 0.5N_\beta\}$ [17][19][20]. The k-space part of the total energy of dipole-dipole interaction follows from Eq. (S1) where the continuous variables have been replaced by their discreet analogues:

$$U^{(k)} = \frac{1}{2V}\sum_{\mathbf{k}_\mathrm{n}\neq 0}\left|\hat{\boldsymbol{\rho}}_{\mathbf{k}_\mathrm{n}}\cdot i\mathbf{k}_\mathbf{n}\right|^2\hat{G}'_{\mathbf{k}_\mathbf{n}} - \frac{2\alpha^3}{3\sqrt{\pi}}\sum_{i=1}^{N}\boldsymbol{\mu}_i^2$$

The potential is computed at each mesh point $\mathbf{r}_m$ by

$$\phi_{\mathbf{r}_m}^{(k)} = \frac{1}{V}\mathrm{FFT}^{-1}\{\hat{\phi}_{\mathbf{k}_n}\}(\mathbf{r}_m)$$

where $\hat{\phi}_{\mathbf{k}_n} = \hat{\boldsymbol{\rho}}_{\mathbf{k}_n}\hat{G}'_{\mathbf{k}_n}$. The reciprocal electrostatic field at each mesh point $\mathbf{r}_m$: $\mathbf{E}_{\mathbf{r}_m}^{(k)} = \mathrm{FFT}_{\mathbf{k_n}\neq 0}^{-1}\left\{\hat{\mathbf{E}}_{\mathbf{k}_n}^{(k)}\right\}(\mathbf{r}_m)$ is calculated by differentiating the potential in Fourier space $\hat{\mathbf{E}}_{\mathbf{k}_n}^{(k)} = i\mathbf{k_n}\left[\hat{\boldsymbol{\rho}}_{\mathbf{k}_n}\cdot i\mathbf{k_n}\right]\hat{G}'_{\mathbf{k}_n}$ using the gradient operator $i\mathbf{k_n}$ [17][18][19]. The back interpolation of mesh-based quantities onto particle positions $\mathbf{r}_i$ is achieved using the assignment functions $W^{(p)}$ [18]

$$X^{(k)}(\mathbf{r}_i) = \sum_{\mathbf{r}_m} X_{\mathbf{r}_m}^{(k)} W^{(p)}(\mathbf{r}_m - \mathbf{r}_i)$$

The **k**-space torque on dipole *i* is computed from the electric field obtained at the position of the dipole

$$\boldsymbol{\tau}_i^{(k)} = \boldsymbol{\mu}_i \times \mathbf{E}^{(k)}(\mathbf{r}_i)$$

Likewise, the **k**-space force on each dipole [17]

$$\mathbf{F}_i^{(k)} = \sum_{\mathbf{r}_m} W(\mathbf{r}_m - \boldsymbol{r}_i)\{\hat{\mu}_{i,x}\mathrm{FFT}_{\mathbf{k_n}\neq 0}^{-1}\left[\hat{E}_{\mathbf{k}_n,x} i\mathbf{k_n}\right] + \hat{\mu}_{i,y}\mathrm{FFT}_{\mathbf{k_n}\neq 0}^{-1}\left[\hat{E}_{\mathbf{k}_n,y} i\mathbf{k_n}\right] + \hat{\mu}_{i,z}\mathrm{FFT}_{\mathbf{k_n}\neq 0}^{-1}\left[\hat{E}_{\mathbf{k}_n,z} i\mathbf{k_n}\right]\}(\mathbf{r_p})$$

The lattice Green function $\hat{G}'_{\mathbf{k_n}}$ is introduced in an optimized form, which minimizes the discretization errors [17][19]

$$\hat{G}'_{\mathbf{k_n}} = \frac{\sum_{\mathbf{m}}[i\mathbf{k_n}\cdot i\mathbf{k_m}]^s \hat{U}_{\mathbf{k_m}}^2 \hat{G}(\mathbf{k_m})}{[i\mathbf{k_n}]^{2s}\left(\sum_{\mathbf{m}}\hat{U}_{\mathbf{k_m}}^2\right)^2}$$

where $\mathbf{k_m} \equiv \{\mathbf{k_n} + 2\pi(\mathbf{Nm})^T\mathbf{a}^{-1}\text{: } \mathbf{m} \in \mathbb{Z}^3\}$ (the sum over $\mathbf{m}$ converges quickly) [20], $\hat{U}_{\mathbf{k}} = \frac{1}{|\mathbf{H}|}\hat{W}_{\mathbf{k}}$ and $\hat{W}_{\mathbf{k}} = \int_V e^{i\mathbf{k}\cdot\mathbf{r}} W(\mathbf{r})\, d^3\mathbf{r} = |\mathbf{H}|\left[\prod_\beta \mathrm{sinc}\left(\frac{\pi n_\beta}{N_\beta}\right)\right]^p$ is the Fourier transform of the assignment function. The exponent S = 3 is used for the force and stress calculation and S = 2 - for the energy, electric field and torque. In the case of changeable simulation box size/shape the lattice Green function is recomputed at each time step.

*Virial stress*. In NPT simulations the volume of the simulation box must change in response to the imbalance of the internal/external stress, which has a direct and reciprocal terms due to the **k**-space splitting of the electric field contributions. For the direct part of the virial stress increment based on a short-ranged pair-wise potential a standard expression is suitable [15][21]

$$\Delta\Pi_{\alpha\beta}^{(r)} = \frac{1}{2V}\sum_{\mathbf{n}\in\mathbb{Z}^3}{}^{\prime}\sum_{i=1}^{N}\sum_{j=1}^{N}\left(\mathbf{r}_{ij\mathbf{n}}\right)_\alpha\left(\mathbf{F}_{ij\mathbf{n}}^{(r)}\right)_\beta$$

The reciprocal contribution is developed following the approach of Andersen [22], Smith [14], Parrinello and Rahman [23], Nose and Klein [24] where the **k**-space term $\Pi_{\alpha\beta}^{(k)}$ is deduced from the energy scaling relation [24][25]

$$-\frac{\partial U^{(k)}(\{\vec{s}_i\},\boldsymbol{a})}{\partial a_{\alpha\beta}} = V\sum_\gamma \Pi^{(k)}_{\alpha\gamma} a^{-1}_{\beta\gamma} \quad \text{(S2)}$$

Here, $U^{(k)}(\{\vec{s}_i\},\boldsymbol{a})$ is the reciprocal part of the potential energy of the simulation cell. Using Eq. (S1) and geometric relations $\frac{\partial V}{\partial a_{\alpha\beta}} = V(\boldsymbol{a}^{-1})_{\beta\alpha}$ (*via* Jacobi's formula), $\frac{\partial k_\gamma}{\partial a_{\alpha\beta}} = -k_\alpha a^{-1}_{\beta\gamma}$ the application of Eq. (S2) to the **k**-space part of the potential energy produces the reciprocal virial as the sum $\boldsymbol{\Pi}^{(\boldsymbol{k})} = \boldsymbol{\Pi}^{(\mathbf{0})} + \boldsymbol{\Pi}^{(\mathbf{1})}$ of a monopolar contribution

$$\Pi^{(0)}_{\alpha\beta} = \frac{1}{2V^2}\sum_{\mathbf{k_n}\neq 0}\left[\delta_{\alpha\beta} - 2(\mathbf{k_n})_\alpha(\mathbf{k_n})_\beta\left(\frac{1}{k_n^2}+\frac{1}{4\eta^2}\right)\right]\left|i\mathbf{k_n}\cdot\hat{\boldsymbol{\rho}}_{\mathbf{k}_n}\right|^2 \hat{G}'_{\mathbf{k_n}}$$

which originates from the $\boldsymbol{a}$-dependence of the volume V and of the kernel [24][25][26], and a dipolar one

$$\Pi^{(1)}_{\alpha\beta} = \frac{1}{V^2}\sum_{\mathbf{k_n}\neq 0}(\mathbf{k_n})_\alpha\left(\hat{\boldsymbol{\rho}}_{\mathbf{k}_n}\right)_\beta\left(\mathbf{k_n}\cdot\hat{\boldsymbol{\rho}}_{-\mathbf{k}_n}\right)\hat{G}'_{\mathbf{k_n}}$$

Which comes from the $\boldsymbol{a}$-dependence of the kernel and is similar to that reported before [15][27], but where the Fourier mesh vectors, dipole density and the influence function have been replaced by their discreet analogues.

We have implemented the **k**-space energy, force, torque and virial stress calculations for the dipolar $P^3M$ within the *Highly Optimized Object-Oriented Many particle Dynamics* (HOOMD-blue) framework, which is a general-purpose particle simulation toolkit optimized for performance on NVIDIA GPUs [28][29][30].

*Error estimates and validation*. *A priori* RMS error estimates for $P^3M$ dipolar force within randomly distributed ensembles of dipoles were previously derived by Cerda et al. [17][19] as a sum of direct and reciprocal contributions

$$(\Delta F)^2 = \left(\Delta F^{(r)}\right)^2 + \left(\Delta F^{(k)}\right)^2$$

where

$$\left(\Delta F^{(r)}\right)^2 = \frac{M^4}{N}\frac{1}{V\alpha^4 r_c^9}\left(\frac{13}{6}C_c^2 + \frac{2}{15}D_c^2 - \frac{13}{15}C_c D_c\right)e^{-2\alpha^2 r_c^2}$$

$$\left(\Delta F^{(k)}\right)^2 = \frac{M^4}{N}\frac{\alpha}{9V^2}\sum_{\mathbf{k_n}\neq 0}\left\{\sum_{\mathbf{m}}|\mathbf{k_m}|^6\hat{G}^2(\mathbf{k_m}) - \frac{\left[\sum_{\mathbf{m}}(\mathbf{k_n}\cdot\mathbf{k_m})^3\hat{U}^2_{\mathbf{k_m}}\hat{G}(\mathbf{k_m})\right]^2}{\mathbf{k}_\mathbf{n}^6\left(\sum_{\mathbf{m}}\hat{U}^2_{\mathbf{k_m}}\right)^2}\right\}$$

$$C_c = 4\alpha^4 r_c^4 + 6\alpha^2 r_c^2 + 3$$

$$D_c = 8\alpha^6 r_c^6 + 20\alpha^4 r_c^4 + 30\alpha^2 r_c^2 + 15$$

These estimates are used to guide the Ewald splitting parameter $\alpha$ towards the maximum accuracy (lowest error) of the scheme within an iterative procedure. The error $\Delta F$ calculations for a system of 100 unit dipoles, which are randomly distributed within a simulation cube of length L=10 and using

a real-space cut-off radius $r_c = 4$, i.e. a system identical to the one studied by Cerda et al. [17], is shown in Fig. S1 and fairly accurately reproduces their results.

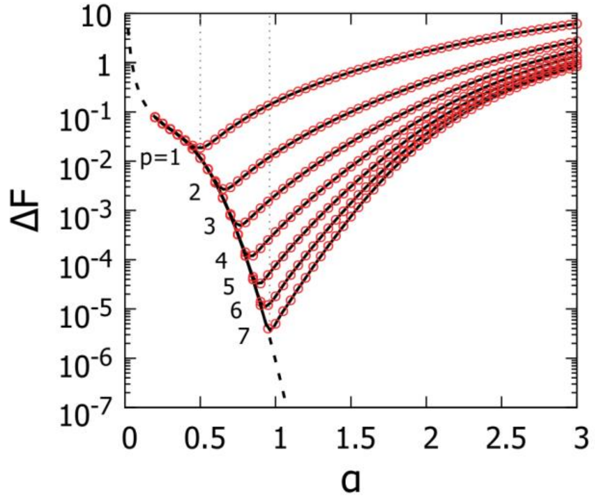


Fig. S1. Calculated RMS error $\Delta F$ for dipolar forces in a system of randomly distributed 100 unit dipoles as a function of Ewald splitting parameter $\alpha$. The dashed line shows the real space contribution $\Delta F^{(r)}$, the solid line indicates the results of Cerda et al. [17].

The correct calculation of potential energies, forces, torques and virial stress within our implementation of $P^3M$ has been verified by series of independent simulations using dipolar Ewald summation [15] with the *Large-scale Atomic/Molecular Massively Parallel Simulator* (LAMMPS) [31] for an identical system. The results agree within the expected precision.

**Self-assembly simulations**

Excluded volume interactions of cubic nanocrystals were modelled using discrete element method (DEM). Simulations of osmotic self-assembly of *N*=15 625 dipolar cubes were carried out using DEM/$P^3M$ dynamics in a periodic simulation box under the isothermal-isobaric NPT ensemble using Martyna-Tobias-Klein hybrid scheme (barostat-thermostat) [32] to produce solid morphologies for characterization. The nominal cube edge length is $\sigma^* = 1$, the simulation time unit is $\tilde{t} = \sqrt{\beta m \sigma^2}$, where $\beta = \frac{1}{kT}$. The starting configurations are disordered low density gas-like states initialized with pseudorandom positions and orientations and initial velocities sampled from the Maxwellian distribution at nominal temperature $T^* = 1$. After a brief thermalization the compression runs simulate the entire self-assembly process from a dilute suspension to a high-density state. We start with a pre-compression ($2{\cdot}10^5$ timesteps, $\Delta t = 0.0005\tilde{t}$) to impose the initial confinement with target density $\phi \approx 0.45$ and facilitate nucleation, then the system is compressed $0.45 < \phi \to 1$ for $2{\cdot}10^6$ timesteps by slowly ramping up the pressure and allowing the system to relax for $10^4$ timesteps after each incremental pressure jump. This is sufficient to form an ordered state of simple cubes in accord with the experiments by Mimura and Kato. After equilibrating the solid phase at target pressure for at least $5{\cdot}10^5$ timesteps, the production run proceeds for $5{\cdot}10^5$ timesteps to collect data and measure the statistical descriptors. The simulations of dipolar cubes are performed by assigning $\langle 001 \rangle$ dipoles (pointing towards cube faces) to the nanocubes with dipolar interaction strength $\lambda = \beta U_{dd} = 0 \div 20$ varying in the indicated range. The isotropy of the stress tensor is verified in each run. The state data is collected from at least 4 to 8 independent trajectories for each state point, uncertainty is reported as

the standard deviation. Since the DEM cubes are slightly larger than their hard cores due to the presence of elastic layer, we rescale the volume and density by an effective edge length ($\sigma_{eff}^{*} \approx 1.1$) determined as the minimum distance of approach from the pair probability distribution function $g_2(r)$, which quantifies the effective excluded volume. The simulations were performed with a *HOOMD-blue* code maintained by the University of Michigan [28][29], which was modified as described above. All calculations were run on the *LASC* cluster of the Institute of Solid State Physics of the University of Latvia.

**Data analysis**

The degree of global orientational order is measured using the cubatic order parameter $P_4 \in [0,1]$, which is sensitive to the 4-fold symmetries of the cubic lattice [33][34]:

$$P_4 = \frac{1}{14}\langle 35\left(\mathbf{u}_{ij}\cdot\mathbf{n}\right)^4 - 30\left(\mathbf{u}_{ij}\cdot\mathbf{n}\right)^2 + 3\rangle$$

Here $\mathbf{u}_{ij}$ is a set of unit vectors along a relevant particle axes and $\mathbf{n}$ is a unit director, which maximizes $P_4$, and is calculated by sampling from a sufficiently large trial set [34]. The averaging $\langle \dots \rangle$ is performed over all 15625 cubes in the ensemble. The positional extent of the mesoscale cubatic correlations is assessed by orientational correlation function $G_4(r) \in [0,1]$, which quantifies the mutual alignment of particles as a function of their separation distance $r$ [34] favoring face-to-face ordering of the cubic lattice: $G_4(r) = \frac{3}{14}\langle 35\left[\mathbf{u}_{i\alpha}(0)\cdot\mathbf{u}_{j\alpha}(r)\right]^4 - 30\left[\mathbf{u}_{i\alpha}(0)\cdot\mathbf{u}_{j\alpha}(r)\right]^2 + 3\rangle$, where $\langle \dots \rangle$ denotes the ensemble average over all particle pairs $(i,j)$ and cube face normals $\alpha$.

The degree of crystalline order in the generated solids is identified with the help of diffraction patterns and polyhedral template matching following literature procedures [35][36][37]. The virtual SAD patterns are calculated along the cubatic director $\mathbf{n}$ of $P_4$, which identifies a high symmetry axis. Polyhedral template matching (PTM) [36][35] is used to assign the crystalline structure by graph-based matching of the convex hull formed by the local neighborhood to a set of predefined reference templates. The spectrum of the root-mean-square deviation ($RMSD \in [0,1]$) of the structure from a set of standard reference lattices is a measure of the local particle environment. The PTM has this advantage that it characterizes order on a local scale and can be used to identify locally ordered regions. To calculate local packing fraction $\Phi^{loc}$ distribution in the consolidated assemblies of nanocubes the indicator function $I_\Phi$, which is equal to 1 within the solid phase X and 0 in the porous space $\Omega$, is defined

$$I_\Phi(\mathbf{r}) = \begin{cases} 0 & \mathbf{r} \in \Omega \\ 1 & \mathbf{r} \in \mathrm{X} \end{cases}$$

The indicator function $I_\Phi$ is mapped onto a fine regular mesh spanning the assembly and the packing topography is generated by coarse graining the meshed distribution $\Phi^{loc}(\mathbf{r}) = \frac{1}{V}\int_{\mathrm{V}(\mathbf{x})} I_\Phi(\mathbf{x})d\mathbf{x}$ respecting the periodicity of the system, where $\mathrm{V}(\mathbf{x}) \sim \sigma^3$ denotes a spherical volume centered at $\mathbf{x}$. The locally orientationally ordered clusters in assemblies without long-range cubatic order are identified using local cubatic order parameter $P_4^{loc}$, which is defined similar to Liu et al. [38]. To that end the simulation domain is discretized by a $\mathbf{N} \equiv \mathrm{diag}(N_1, N_2, N_3)$ mesh, where the mesh points are identified by lattice vectors $\mathbf{r}_{\boldsymbol{m}} \equiv \left\{(\mathbf{aN}^{-1})\mathbf{n} : \mathbf{n} \in \mathbb{Z}^3, 0 \le n_\beta < N_\beta\right\}$. Then $P_4^{loc}(\mathbf{r}_{\boldsymbol{m}}) = \frac{1}{14}\langle 35\big(\mathbf{u}_{ij}\,\cdot$

$\mathbf{n})^4 - 30(\mathbf{u}_{ij} \cdot \mathbf{n})^2 + 3\rangle_{V_\varepsilon(\mathbf{r}_m)}$, where the subscript indicates that the ensemble average is obtained over the particles with centroids within a volume $V_\varepsilon(\mathbf{r}_m)$ in the vicinity of mesh point $\mathbf{r}_m$ as a measure of the local neighborhood. The volume $V_\varepsilon(\mathbf{r}_m)$ encompasses the first two coordination spheres of a perfect cubic lattice calculated from the pair-probability distribution $g_2(r)$. Small ordered cubic packing can be reliably identified in the absence of global order inspecting the locality of packing fraction and local cubatic order. To emulate the surface morphologies the produced ensembles are periodically replicated from the final frames of self-assembly simulations and sliced along high-symmetry axes – the cubatic directors. To calculate the topology of the pair probability distribution [39] and the potential of mean force and torque (PMFT) [40][41] at varying levels of confinement an additional series of NVT simulations are performed branching from the NPT compression trajectories after reaching the desired density. After equilibrating for $10^6$ timesteps the production runs for $10^6$ timesteps. The relative displacements of all pairs of particles within a spherical cutoff are recorded and binned using a regular mesh $\mathbf{r}_m$ with desired resolution in the coordinate system of the first particle (the possible orientations of the second (probe) particle are implicitly integrated, which allows a direct visualization). The spatial distribution of the normalized frequency of occupancy of the bins produces the topology of $g_2(\mathbf{r}_m)$ [39], whereas its logarithm yields the PMFT [40][41]. The simulated trajectories were inspected using the *Open Visualization Tool* (OVITO) [35]. The statistical descriptors were measured from the calculated trajectories as described above, *ParaView* [42] - an open-source, multi-platform data analysis and visualization suite – was used to inspect the produced topological data.

## References


[1] Dovesi, R.; Orlando, R.; Erba, A.; Zicovich-Wilson, C. M.; Civalleri, B.; Casassa, S.; Maschio, L.; Ferrabone, M.; De La Pierre, M.; D'Arco, P., et al. CRYSTAL14: A Program for the Ab Initio Investigation of Crystalline Solids. Int. J. Quantum Chem. 2014, 114, 1287–1317.

[2] Adamo, C.; Barone, V. Toward Reliable Density Functional Methods without Adjustable Parameters: The PBE0 Model. J. Chem. Phys. 1999, 110, 6158–6170.

[3] Mahmoud, A.; Erba, A.; El-Kelany, Kh. E.; Rerat, M.; Orlando, R. Low-Temperature Phase of BaTiO3: Piezoelectric, Dielectric, Elastic, and Photoelastic Properties from Ab Initio Simulations. Phys. Rev. B 2014, 89, 045103.

[4] Erba, A.; El-Kelany, Kh. E.; Ferrero, M.; Baraille, I.; Rerat, M. Piezoelectricity of SrTiO3: An Ab Initio Description. Phys. Rev. B 2013, 88, 035102

[5] Rusevich, L.L., Zvejnieks, G., Erba, A., Dovesi, R., Kotomin, E.A. Electromechanical Properties of $Ba_{(1-x)}Sr_xTiO_3$ Perovskite Solid Solutions from First-Principles Calculations. J. Phys. Chem. A 2017, 121, 9409-9414.

[6] Hay, P.J.; Wadt, W.R. Ab Initio Effective Core Potentials for Molecular Calculations. Potentials for the Transition Metal Atoms Sc to Hg. J. Chem. Phys. 1985, 82, 270–283.

[7] Wadt, W.R.; Hay, P.J. Ab Initio Effective Core Potentials for Molecular Calculations. Potentials for Main Group Elements Na to Bi. J. Chem. Phys. 1985, 82, 284–298.

[8] Hay, P.J.; Wadt, W.R. Ab Initio Effective Core Potentials for Molecular Calculations. Potentials for K to Au Including the Outermost Core Orbitals. J. Chem. Phys. 1985, 82, 299–310.

[9] Piskunov, S.; Heifets, E.; Eglitis, R. I.; Borstel, G. Bulk Properties and Electronic Structure of SrTiO3, BaTiO3, PbTiO3 Perovskites: an Ab Initio HF/DFT Study. Comput. Mater. Sci. 2004, 29, 165–178.

[10] Bredow, T.; Jug, K.; Evarestov, R. A. Electronic and Magnetic Structure of ScMnO3. Phys. Stat. Sol. (b) 2006, 243, R10–R12.

[11] S. Piskunov, E.A. Kotomin, E. Heifets, J. Maier, R.I. Eglitis, G. Borstel. Hybrid DFT calculations of the atomic and electronic structure for ABO3 perovskite (001) surfaces. Surf. Sci. 2005, 575, 75–88.

[12] J.-J. Weis and D. Levesque, in Advanced Computer Simulation Approaches for Soft Matter Sciences II, Springer-Verlag, pp. 163–225

[13] S. W. de Leeuw, J. W. Perram and E. R. Smith, Simulation of Electrostatic Systems in Periodic Boundary Conditions. I. Lattice Sums and Dielectric Constants, Proc. Royal Soc. A, 1980, 373, 27–56.

[14] W. Smith, Point Multipoles in the Ewald Summation, CCP5 Quarterly 4, 13 1982.

[15] A. Toukmaji, C. Sagui, J. Board and T. Darden, Efficient particle-mesh Ewald based approach to fixed and induced dipolar interactions, J. Chem. Phys., 2000, 113, 10913–10927.

[16] Z. Wang and C. Holm, Estimate of the cutoff errors in the Ewald summation for dipolar systems, J. Chem. Phys., 2001, 115, 6351–6359.

[17] J. J. Cerdà, V. Ballenegger, O. Lenz and C. Holm, P3M algorithm for dipolar interactions, J. Chem. Phys., 2008, 129, 234104.

[18] Hockney, R. & Eastwood, J. (1988). *Computer simulation using particles*. Bristol England Philadelphia: A. Hilger.

[19] J. J. Cerdà, V. Ballenegger and C. Holm, Particle-particle particle-mesh method for dipolar interactions: On error estimates and efficiency of schemes with analytical differentiation and mesh interlacing, J. Chem. Phys., 2011, 135, 184110.

[20] V. Ballenegger, J. J. Cerdà and C. Holm, How to Convert SPME to P3M: Influence Functions and Error Estimates, J. Chem. Theory Comput., 2012, 8, 936–947.

[21] A. P. Thompson, S. J. Plimpton and W. Mattson, General formulation of pressure and stress tensor for arbitrary many-body interaction potentials under periodic boundary conditions, J. Chem. Phys., 2009, 131, 154107.

[22] H. C. Andersen, Molecular dynamics simulations at constant pressure and/or temperature, J. Chem. Phys., 1980, 72, 2384–2393.

[23] M. Parrinello and A. Rahman, Crystal Structure and Pair Potentials: A Molecular-Dynamics Study, Phys. Rev. Lett., 1980, 45, 1196–1199.

[24] S. Nosé and M. L. Klein, Constant pressure molecular dynamics for molecular systems, Mol. Phys., 1983, 50, 1055–1076.

[25] N. Karasawa and W. A. Goddard, Acceleration of convergence for lattice sums, J. Phys. Chem., 1989, 93, 7320–7327.

[26] D. Brown and S. Neyertz, A general pressure tensor calculation for molecular dynamics simulations, Mol. Phys., 1995, 84, 577–595.

[27] C. Sagui, L. G. Pedersen and T. A. Darden, Towards an accurate representation of electrostatics in classical force fields: Efficient implementation of multipolar interactions in biomolecular simulations, J. Chem. Phys., 2004, 120, 73–87.

[28] J. A. Anderson, C. D. Lorenz and A. Travesset, General purpose molecular dynamics simulations fully implemented on graphics processing units, J. Comput. Phys., 2008, 227, 5342–5359.

[29] J. Glaser, T. D. Nguyen, J. A. Anderson, P. Lui, F. Spiga, J. A. Millan, D. C. Morse and S. C. Glotzer, Strong scaling of general-purpose molecular dynamics simulations on GPUs, Comput. Phys. Commun., 2015, 192, 97–107

[30] D. N. LeBard, B. G. Levine, P. Mertmann, S. A. Barr, A. Jusufi, S. Sanders, M. L. Klein and A. Z. Panagiotopoulos, Self-assembly of coarse-grained ionic surfactants accelerated by graphics processing units, Soft Matter, 2012, 8, 2385–2397.

[31] S. Plimpton, Fast Parallel Algorithms for Short-Range Molecular Dynamics, J. Comput. Phys., 1995, 117, 1–19.

[32] J. Martyna, D. J. Tobias and M. L. Klein, Constant pressure molecular dynamics algorithms, J. Chem. Phys., 1994, 101, 4177–4189.

[33] U. Agarwal and F. A. Escobedo, Mesophase behaviour of polyhedral particles, Nat. Mater., 2011, 10, 230–235.

[34] R. D. Batten, F. H. Stillinger and S. Torquato, Phase behavior of colloidal superballs: Shape interpolation from spheres to cubes, Phys. Rev. E, 2010, 81, 061105.

[35] A. Stukowski, Visualization and analysis of atomistic simulation data with OVITO–the Open Visualization Tool, Modelling and Simulation in Materials Science and Engineering, 2009, 18, 15012.

[36] P. M. Larsen, S. Schmidt and J. Schiøtz, Robust structural identification via polyhedral template matching, Modelling and Simulation in Materials Science and Engineering, 2016, 24, 55007.

[37] S. P. Coleman, D. E. Spearot and L. Capolungo, Virtual diffraction analysis of Ni [0 1 0] symmetric tilt grain boundaries, Modelling and Simulation in Materials Science and Engineering, 2013, 21, 55020.

[38] L. Liu, Z. Li, Y. Jiao and S. Li, Maximally dense random packings of cubes and cuboids via a novel inverse packing method, Soft Matter, 2017, 13, 748–757.

[39] D. Zablotsky, E. Blums and H. J. Herrmann, Self-assembly and rheology of dipolar colloids in simple shear studied using multi-particle collision dynamics, Soft Matter, 2017, 13, 6474–6489.

[40] G. van Anders, D. Klotsa, N. K. Ahmed, M. Engel and S. C. Glotzer, Understanding shape entropy through local dense packing, Proceedings of the National Academy of Sciences, 2014, 111, E4812–E4821.

[41] G. van Anders, N. K. Ahmed, R. Smith, M. Engel and S. C. Glotzer, Entropically Patchy Particles: Engineering Valence through Shape Entropy, ACS Nano, 2013, 8, 931–940.

[42] Ahrens, J., Geveci, B., Law, C., *ParaView: An End-User Tool for Large Data Visualization, Visualization Handbook*, Elsevier, 2005, ISBN-13: 978-0123875822
